# Supplementary material for: Set-of-Mark Prompting Unleashes Extraordinary Visual Grounding in GPT-4V
Source: arXiv:2310.11441 source file (2023-11-06)
Supplement: Supplementary file 1 [file case_2.tex]

\begin{figure}

\centering
    \begin{AIbox}{Task Planning}
\begin{minipage}{\textwidth}
\begin{minipage}{0.48\linewidth}
    \footnotesize
    \textbf{\textcolor{Orange}{User}}: How to make coffee with this machine?
    \\
    \\
    \\
    \\
    \\
\end{minipage}
\hfill
\begin{minipage}{0.48\linewidth}
    \includegraphics[width=\linewidth]{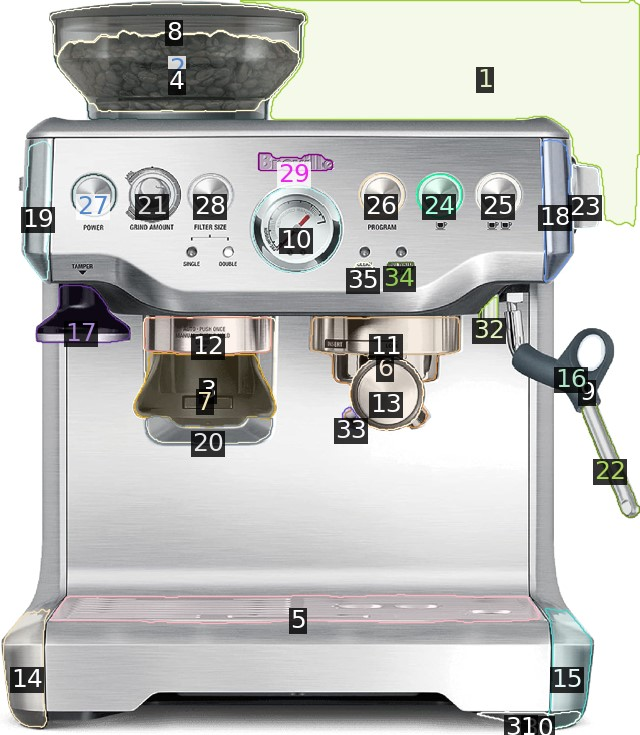}        
\end{minipage}
\end{minipage}
\begin{minipage}{\textwidth}
\textbf{\textcolor{Purple}{GPT-4V~(SoM)}}: 
\\
\\
\footnotesize
The image you provided depicts an espresso machine with various labeled parts. While I don't have the exact manual for this specific machine, based on the standard features of many espresso machines and the labeled components in the image, I can provide you with a general guide on how to make coffee:
\\
\begin{itemize}[leftmargin=*]
\item Water Reservoir (1): Ensure the water reservoir is filled with fresh water. Depending on the capacity of the reservoir, this will dictate how many cups of coffee or espresso you can make before needing to refill.

\item Bean Hopper (8): Ensure the bean hopper is filled with coffee beans. The grinder will use these to produce fresh coffee grounds.

\item Power Button (19): Turn on the machine using the power button. \xyz{power button seems to be wrong}

\item Grind Amount (27) \xyz{it is power}: Adjust the grind amount based on how strong you want your coffee. More grounds typically mean a stronger coffee.

\item Filter Size (28): Choose between a single or double shot. This often corresponds to the size of the filter basket you're using inside the portafilter.

\item Grinding (21): Once you've selected your grind amount and filter size, you can initiate the grinding process, which will deposit the coffee grounds into the portafilter.

\item Tamping (17): After grinding, you'll need to tamp the coffee grounds in the portafilter. This ensures an even extraction when the hot water passes through the coffee.

\item Portafilter (11): Insert the portafilter into the machine's group head.

\item Brewing: Initiate the brewing process using the relevant button. It could be one of the buttons (24, 25, 26) or the central dial (10). Watch as the coffee extracts into your cup placed underneath.

\item Steam Wand (16): If you're making a cappuccino or latte, you can use the steam wand to froth your milk. Make sure to immerse the tip of the wand just below the milk's surface and turn it on. This will introduce air into the milk, creating a creamy froth.

\item Cleaning: After each use, especially after using the steam wand, ensure that you clean the machine parts properly. The drip tray (14) and the used grounds bin (20) should be emptied and cleaned regularly.
\end{itemize}
Keep in mind, for specific functions or nuances, you'll need to refer to the machine's user manual. If you have that, it would provide the most accurate step-by-step guide for this particular model. Otherwise, the above is a general guide based on the labeled components in the image.
\end{minipage}
\end{AIbox}   
\label{fig:case_2}
\caption{SoM-prompted GPT-4V does a reasonably good job of doing task planning and grounding the instructions to the image, which are crucial in realistic scenarios if a user does not know the machine.}
\end{figure}
