# Supplementary material for: Set-of-Mark Prompting Unleashes Extraordinary Visual Grounding in GPT-4V
Source: arXiv:2310.11441 source file (2023-11-06)
Supplement: Supplementary file 2 [file som_tittle1.pdf]

Input: Image

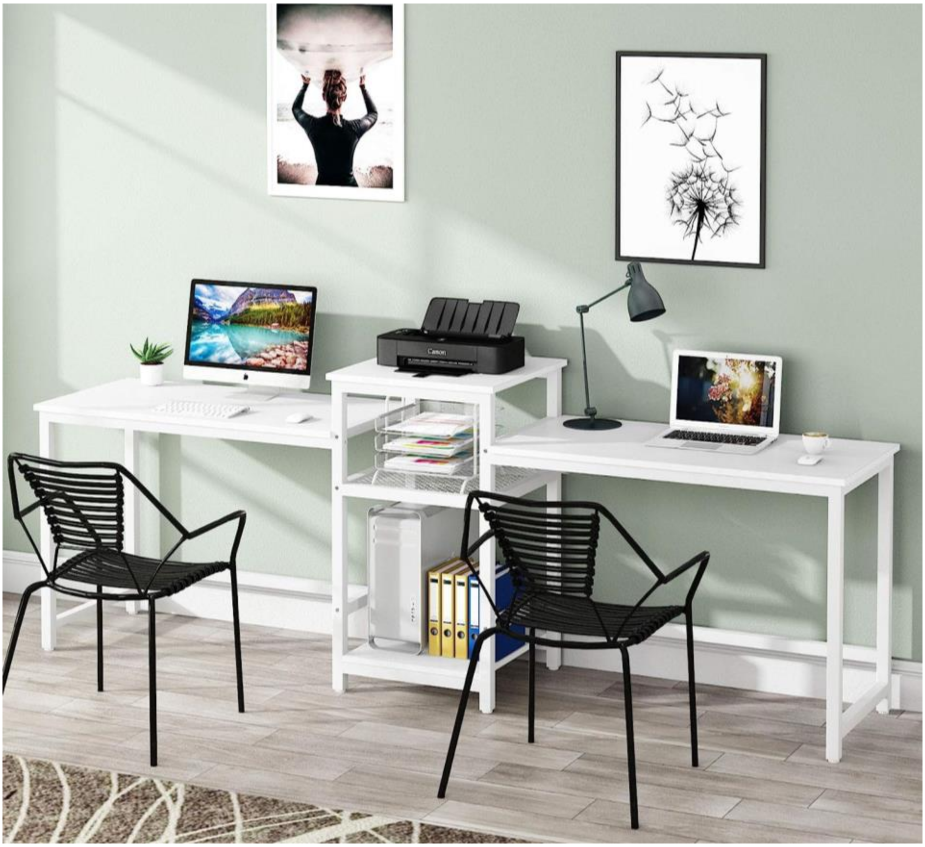

Conversation

| | |
|---|---|
| **User** | What is on the left side of the right laptop? |
| **GPT-4V** | On the left side of the right laptop, there is a **cup or mug**. ✗ |
| **User** | I want to find a seat close to windows, where can I sit? |
| **GPT-4V** | You can sit on **either of the two black chairs** in front of the white desks, as they are closest to the windowed wall. ✗ |

Input: Image + SoM

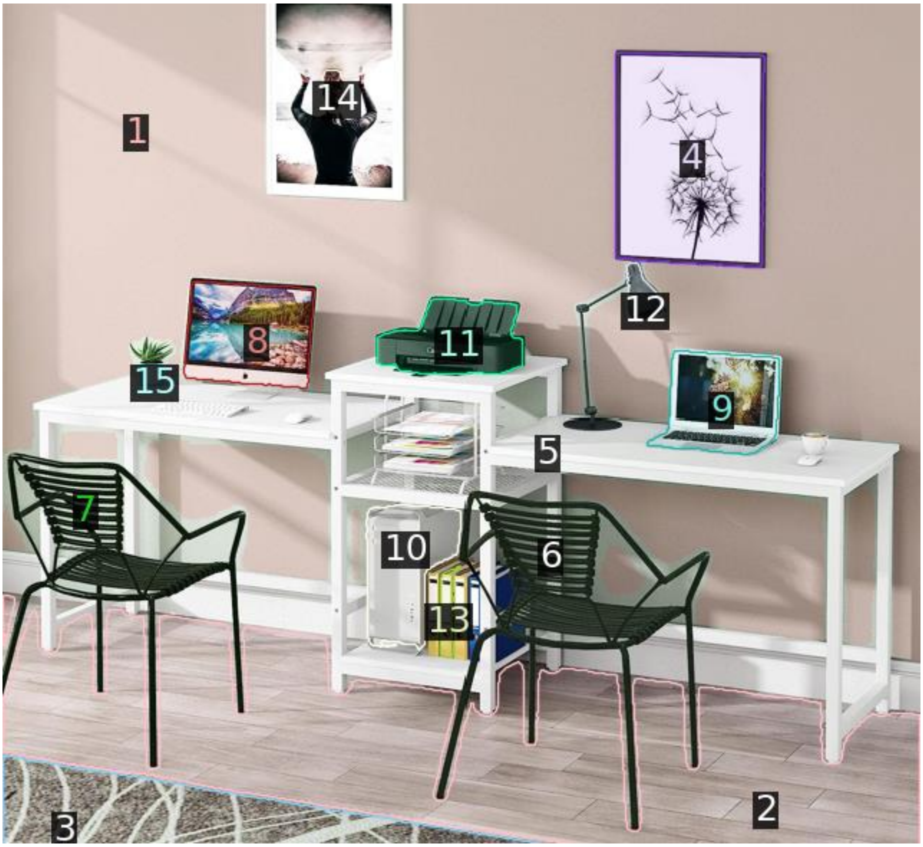


Conversation

| | |
|---|---|
| **User** | What is on the left side of the right laptop? |
| **GPT-4V** | On the left side of the right laptop (numbered as 9), there is **a lamp, which is numbered as 12**. ✓ |
| **User** | I want to find a seat close to windows, where can I sit? |
| **GPT-4V** | You can sit on the **chair numbered as 7**. It's the closest seat to the windows (represented by the area numbered as 1). ✓ |
